# Supplementary material for: NavRep: Unsupervised Representations for Reinforcement Learning of Robot Navigation in Dynamic Human Environments
Source: arXiv:2012.04406 source file (2020-12-08)
Supplement: Supplementary file 1 [file appendix.tex]

\section*{APPENDIX}
\subsection{Training parameters}

\subsection{"Dream" results}

\subsection{Detailed results}
\begin{table*}
\scriptsize
\caption{Per-scenario success rates [\%] in unseen environments}
\vspace{-10pt}
\label{tab:nudge-results-ttg}
\setlength\tabcolsep{3pt}
\begin{center}
% start of pasted text ---
\begin{tabular}{ c c c c c c c c c c c c c c c c c c c c c c c c c c c c}
\toprule
& \multicolumn{9}{c}{simple} & \multicolumn{9}{|c|}{complex} & \multicolumn{9}{c}{realistic} \\
& 1    & 2    & 3    & 4    & 5    & 6    & 7    & 8    & 9    & 1    & 2    & 3    & 4    & 5    & 6    & 7    & 8    & 9    & 1    & 2    & 3    & 4    & 5    & 6    & 7    & 8    & 9    \\
\midrule
End-to-end (1D) &       66.7 &        4.9 & \textbf{9.3} & \textbf{7.5} &       88.9 & \textbf{59.3} & \textbf{100.0} & \textbf{99.0} &        4.9 &       42.9 &        8.7 &        3.4 &        0.0 &       39.9 &       76.3 &       99.7 &       93.2 &       34.0 &        0.0 &        0.0 &        0.0 &        0.0 &        0.0 &        0.0 &        0.8 &        0.0 &        2.1 \\
End-to-end &       30.7 &       19.6 &        5.4 &        0.5 &       69.3 &       43.6 &       98.3 &       63.8 &       57.0 & \textbf{84.7} &       15.5 & \textbf{10.9} &        0.0 &       28.7 & \textbf{78.9} &       99.2 &       81.6 &       46.7 &       10.7 &        3.6 &        0.0 &        0.0 &       85.0 & \textbf{21.4} &       33.8 &       12.0 & \textbf{20.1} \\
SOADRL     &       12.4 &        6.0 &        0.0 &        0.3 & \textbf{94.5} &       40.2 & \textbf{100.0} &       69.0 & \textbf{70.9} &        3.7 &        0.0 &        2.2 &        0.0 &        8.0 &       32.9 & \textbf{100.0} &        1.4 &       46.6 &        0.3 &        0.0 &        0.0 &        0.0 &       43.0 &        1.0 & \textbf{100.0} &        0.0 &       18.8 \\
Modular (1D), z only &        5.3 &        1.3 &        0.0 &        0.0 &       28.6 &       29.9 & \textbf{100.0} &       65.7 &        2.2 &        5.6 &        0.3 &        3.2 &        3.2 &       11.5 &       15.1 &       99.7 &       77.0 &        4.3 &        0.0 &        0.0 &        0.0 &        0.0 &       24.9 &        0.0 &       91.5 &       37.6 &        0.0 \\
Modular (1D), h only &        4.6 &        1.1 &        0.0 &        0.0 &       23.4 &       23.7 & \textbf{100.0} &       80.7 &        2.0 &        1.4 &        1.1 &        8.0 &        0.8 &       10.1 &       11.9 &       93.3 &       69.9 &       15.0 &        0.0 &        0.0 &        0.0 &        0.0 &       22.9 &        0.0 &       98.7 &       78.8 &        0.8 \\
Modular (1D), z+h &        7.9 &        3.9 &        0.0 &        0.0 &       29.6 &       35.1 & \textbf{100.0} &       86.2 &        2.0 &       15.6 &        0.3 &        7.7 &        5.4 &       11.8 &       26.4 & \textbf{100.0} &       83.6 &       13.3 &        0.0 &        0.0 &        0.0 &        0.0 &       29.5 &        0.0 & \textbf{100.0} &       74.9 &        0.5 \\
Joint (1D), z only &        4.3 &        1.0 &        0.0 &        0.0 &       29.7 &       24.1 &       99.7 &       81.4 &        3.2 &        5.2 &        0.3 &        4.1 &        0.0 &       14.0 &       16.1 & \textbf{100.0} &       60.2 &        7.4 &        0.0 &        0.0 &        0.0 &        0.0 &       15.0 &        0.0 &       56.0 &        1.5 &        0.3 \\
Joint (1D), h only &        0.0 &        0.0 &        0.0 &        0.3 &       23.7 &       12.6 & \textbf{100.0} &       68.5 &        1.4 &        0.0 &        0.2 &        2.0 &        0.0 &        4.3 &       17.5 & \textbf{100.0} &        5.4 &        8.6 &        0.0 &        0.0 &        0.0 &        0.0 &       33.9 &        0.8 & \textbf{100.0} &       18.5 &        0.0 \\
Joint (1D), z+h &        0.0 &        0.3 &        0.0 &        0.0 &       19.1 &       27.9 &       97.2 &       85.0 &        2.7 &        1.0 &        0.0 &        2.6 &        0.0 &       10.3 &       23.0 &       99.2 &       84.5 &        8.4 &        0.0 &        0.0 &        0.0 &        0.0 &        9.7 &        0.0 &       53.8 &        0.0 &        0.5 \\
Modular, z only &       33.7 &        1.6 &        0.0 &        0.0 &       36.8 &       39.8 & \textbf{100.0} &       79.9 &        4.9 &       26.3 &        0.9 &        3.8 &        0.0 &       29.8 &       24.2 & \textbf{100.0} & \textbf{100.0} &       19.2 &        6.7 &        4.4 &        0.0 &        0.0 &       60.1 &        1.0 & \textbf{100.0} &       98.5 &        0.5 \\
Modular, h only &       62.2 &       16.8 &        1.1 &        0.0 &       35.6 &       27.9 & \textbf{100.0} &       89.3 &        4.3 &       69.0 &        1.9 &       10.1 & \textbf{11.1} &       24.4 &       35.4 & \textbf{100.0} &       99.7 &       18.4 &        1.3 &        0.0 &        0.3 &        0.0 &       54.6 &        1.6 & \textbf{100.0} & \textbf{100.0} &        0.8 \\
Modular, z+h &       45.1 &       11.8 &        1.3 &        0.3 &       38.7 &       32.5 & \textbf{100.0} &       94.8 &        5.5 &       57.6 &        5.2 &        6.8 &        1.0 &       26.2 &       37.2 & \textbf{100.0} &       95.8 &       17.4 &        8.4 &        1.6 &        0.3 &        0.0 &       53.6 &        1.3 & \textbf{100.0} &       98.9 &        0.3 \\
Joint, z only &       46.4 &       18.4 &        0.2 &        0.8 &       79.4 &       51.1 & \textbf{100.0} &       66.6 &       44.3 &       58.2 & \textbf{21.4} &        8.9 &        0.0 &       61.8 &       61.1 & \textbf{100.0} &       95.9 &       53.4 & \textbf{18.8} & \textbf{6.4} &        0.0 &        0.0 &       97.2 &       12.1 & \textbf{100.0} &       47.9 &        5.6 \\
Transformer, z only & \textbf{75.2} & \textbf{25.5} &        0.5 &        0.3 &       89.3 &       59.1 &       99.5 &       78.6 &       58.7 &       16.9 &       14.4 &        0.0 &        0.0 & \textbf{67.8} &       68.5 &       98.5 &       94.2 & \textbf{53.6} &        3.7 &        5.7 & \textbf{0.3} &        0.0 & \textbf{97.7} &        7.7 &       94.9 &       64.0 &        7.1 \\
\bottomrule
\end{tabular}
% ----- end of pasted text
\vspace{-0.5cm}
\end{center}
\end{table*}

\subsection{extra comparisons (which help justify choices)}
\subsubsection{V32 vs V64}
\subsubsection{GPT 1D ?}
\subsubsection{PPO vs CMA vs ...}
\subsubsection{Adaptive training}
